# Supplementary material for: DOF-GS:Adjustable Depth-of-Field 3D Gaussian Splatting for Post-Capture Refocusing, Defocus Rendering and Blur Removal
Source: arXiv:2405.17351 source file (2025-06-07)
Supplement: Supplementary file 1 [file supp.tex]

\PassOptionsToPackage{table}{xcolor}
\documentclass[10pt, letterpaper]{article}
  \usepackage{cvpr_v3_1}

 % *** Enter the CVPR Paper ID here

% \usepackage{cvpr}      

\input{package_arxiv}
\usepackage{cleveref}
% To produce the CAMERA-READY version
% \usepackage[pagenumbers]{cvpr} 
% \documentclass[acmtog, review, anonymous, timestamp, nonacm]{acmart}
%\documentclass[acmtog, authorversion]{acmart}

\input{package_arxiv}
\input{macros_arxiv}
\input{symbols}
\input{graphicspath}

\includeonly{}
\input{sections/0-title_author}
\begin{document}
\input{hackstyle}

\input{sections/11-supp-title}
\maketitle
\definecolor{bestcolor}{RGB}{255,255,255} % Gold color for best
\definecolor{secondbestcolor}{RGB}{255,255,255} %

% \subsection{Image Deblurring}
% Image deblurring aims to recover a sharp image from a blurred observation caused by diverse sources such as camera shake, object motion, or defocus. Defocus blur, in particular, occurs when objects fall outside the DOF, which is the region around the focal plane where objects appear sharp, \emph{i.e.}, in focus. 
% The blur kernel for defocus blur is spatially-varying and often approximated by Gaussian kernels \cite{shi2015just, xu2017paches} or disk kernels \cite{dandres2016tip, cho2017converge}. Conventional defocus deblurring techniques begin by estimating a defocus map to indicate the extent of blur at each pixel, which then guides the deblurring process. These methods \cite{edge_defocus, shi2015just, unified2017, lee2019defocus} utilize hand-crafted features, deep learning features, or a combination of both for defocus map estimation. However, two-stage workflows can amplify errors from defocus map estimation during deblurring. Recent end-to-end models \cite{son2021single, quan2021gaussian} significantly improve results. Despite the advancements, image deblurring methods risk inducing view inconsistencies in multi-view images.
\section{Derivatives of the differentiable DOF rendering}
In this section, we elaborate on the derivation of key derivatives. Since the majority of the gradient calculations are already incorporated within the customized rasterization process \cite{3dgs}, we focus solely on deriving the derivatives of the gradient pertaining to the affected or newly introduced variables in our differentiable depth-of-field (DOF) rendering process. 
For brevity, we omit the subscript index $m$ for viewpoint.

% Given that the convolution of two Gaussians yields another Gaussian with a covariance matrix equal to the sum of the original Gaussians' covariance matrices \cite{zwicker2001ewa}, we derive the covariance of $\mathcal{G}^{\prime \prime}_{k}$ as follows:
Since the convolution of two Gaussians results in another Gaussian whose covariance matrix is the sum of the covariance matrices of the original Gaussians \cite{zwicker2001ewa}, the covariance of $\mathcal{G}^{\prime \prime}_{k}$ is derived as follows:
\begin{equation}\label{eq:sigma_coc}
    \bm{\Sigma}_{k}^{\prime\prime} = \bm{\Sigma}_{k}^{\prime} + \bm{\Sigma}_{k}^{(\text{coc})} = \begin{bmatrix}
      \bm{\Sigma}_{k}^{\prime}(1,1)+ a & \bm{\Sigma}_{k}^{\prime}(1,2) \\
       \bm{\Sigma}_{k}^{\prime}(2,1) & \bm{\Sigma}_{k}^{\prime}(2,2) + a
    \end{bmatrix}.
\end{equation}
% As the derivatives relative to $\Sigma^{\prime}$ have been provided, we only need to additionally to account for the gradients derived from $\Sigma^{(\text{coc})}$.
By exploiting the chain rule, we can calculate the derivatives w.r.t. focal distance $f$, aperture parameter $Q$ and depth value $z_k$ through the following formulas:
\begin{equation}\label{eq:d_f}
    \frac{d \Sigma^{\prime \prime}_{k}}{d f} = \frac{d \Sigma^{\prime \prime}_{k}}{d \Sigma^{(\text{coc})}_k} \frac{d \Sigma^{(\text{coc})}_k}{d f},
\end{equation}
\begin{equation}
    \frac{d \Sigma^{\prime \prime}_k}{d Q} = \frac{d \Sigma^{\prime \prime}_k}{d \Sigma^{(\text{coc})}_k} \frac{d \Sigma^{(\text{coc})}_k}{d Q},
    % & \frac{d \Sigma^{\prime \prime}}{d A} = \frac{d \Sigma^{\prime \prime}}{d \Sigma^{(\text{coc})}} \frac{d \Sigma^{(\text{coc})}}{d A}, \\ 
\end{equation}
and
\begin{equation}\label{eq:d_z}
     \frac{d \Sigma^{\prime \prime}_k}{d z_k} = \frac{d \Sigma^{\prime \prime}_k}{d \Sigma^{\prime}_k} \frac{d \Sigma^{\prime}_k}{d z_k} + \frac{d \Sigma^{\prime \prime}}{d \Sigma^{(\text{coc})}_k} \frac{d \Sigma^{(\text{coc})}_k}{d z_k}.
\end{equation}
From Equation (\ref{eq:sigma_coc}), the derivative w.r.t. $\Sigma^{\prime}_k$ and $\Sigma^{(\text{coc})}_k$ can be obtained as: $\frac{d \Sigma^{\prime \prime}_k}{d \Sigma^{\prime}_k} = \mathbf{I}$ and $\frac{d \Sigma^{\prime \prime}_k}{d \Sigma^{(\text{coc})}_k} = \mathbf{I}$. For calculating the derivative in Equation (\ref{eq:d_f}), we need to calculate the derivative w.r.t. $f$ from $a$ ($a=\frac{1}{2ln4}\left(R_{k}^{(\text{coc})}\right)^2$), which is given by
\begin{equation}
    \frac{da}{df}=\frac{da}{dR^{(\text{coc})}_k}\frac{dR^{(\text{coc})}_k}{df}=
    \left\{\begin{matrix}
          -\frac{1}{2ln4}\frac{R^{(\text{coc})}_k Q}{f^2},\:\:\: & \text{if\:} z_k>f,\\
          \frac{1}{2ln4}\frac{R^{(\text{coc})}_k Q}{f^2},\:\:\: & \text{otherwise}.
    \end{matrix} \right.
\end{equation}
And the derivative for $Q$ is calculated as 
\begin{equation}
    \frac{da}{dQ}=\frac{R^{(\textbf{coc})}_k}{2ln4}\left|\frac{1}{z_k}-\frac{1}{f}\right|.
\end{equation}
Since $\frac{d\Sigma^{\prime}_k}{dz_k}$ in Equation (\ref{eq:d_z}) has been provided in the rasterization-based rendering of 3DGS \cite{3dgs}, we calculate gradient for $z_k$ by additionally accumulating the derivative w.r.t. $z_k$ relative to $a$: 
\begin{equation}
  \frac{da}{d{z_k}}=
\left\{\begin{matrix}
     -\frac{1}{2ln4}\frac{R^{(\text{coc})}Q}{\left(z_k\right)^2},\:\:\: & \text{if\:} z_k<f,\\
      \frac{1}{2ln4}\frac{R^{(\text{coc})}Q}{\left(z_k\right)^2},\:\:\: & \text{otherwise}.
\end{matrix}\right.  
\end{equation}

% \begin{equation}
% \left\{
% \begin{aligned}
%     \dot{z}_1&=\frac{N\zeta}{t}      &   z_1\left( 0 \right) &=1\\
% 	\zeta &=-G\left( s \right) z_1   &   \zeta \left( 0 \right) &=0\\
% 	\dot{z}_2&=z_1                   &   z_2\left( 0 \right) &=0\\
% 	\dot{z}_u&=z_2                   &   z_u\left( 0 \right) &=0\\
% \end{aligned}
% \right. 
% \end{equation}
\noindent 

In our pipeline, 
 which is designed to learn camera characteristics for the introduced depth-of-field rendering process and to recover scene details from uncalibrated images with moderate defocus blur, we heuristically initialize the focal distance $f$ and aperture parameters $Q$ for each input view and update them through optimization. The initialization strategy is discussed in \Cref{sec:cam_init}. To prevent Gaussian points from being influenced by the focal distance parameters that are actively updated during the optimization process, we disable gradient flow from $\Sigma_k^{(\text{coc})}$ to $z_k$ during the optimization.
% Moreover, to avoid letting focal distance directly affect the positions of Gaussians within the scene, we omit the gradient for $z_{k,m}$ flowed from $a$.

\section{Additional Implementation Details}
In this section, we provide additional implementation details of our approach. Specifically, we outline the initialization of virtual cameras for training views in Section \ref{sec:cam_init}, describe the optimization settings in detail in Section \ref{sec:optimization}, and present further information about parameter settings and the network structure of the In-Focus Localization Network (ILN) in Section \ref{sec:param}.
  
\subsection{Camera Parameter Initialization} \label{sec:cam_init}
As the labels for focal distances $\{f_m\}_{m=1}^{M}$ and aperture parameters $\{Q_m\}_{m=1}^{M}$ across different views are unavailable, an initialization process is required. We simply initialize the focal distances and aperture parameters to be the same value for different views, which avoids a too dedicated manual initialization. Specifically, to avoid introducing bias for focal distances before the optimization, we initialize $f_m$ as the median diopter value among all Gaussian points:
\begin{equation}
    \frac{1}{f_m} = \text{median}\left(\left\{\frac{1}{z_k}\right\}\right),\:\: m=1,2,...,M.
\end{equation}
Initializing $f_m$ to be the median diopter value also helps avoid heavily biased CoC radius values across different depth planes at early iterations. Meanwhile, we initialize the aperture parameter $Q_m$ by ensuring that the CoC values for different points are not greater than a threshold $\tau$. Specifically, the maximum CoC value across the scene occurs at the closest or most distant points when the focal plane is exactly at the opposite side. Thus $Q_m$ is initialized by solving
\begin{equation}
    Q_m\Bigg| \frac{1}{\text{min}\left\{\frac{1}{z_k}\right\}} - \frac{1}{\text{max}\left\{\frac{1}{z_k}\right\}} \Bigg| = \tau,
\end{equation}
which ensures that the most CoC values across the entire scene are not greater than $\tau$. In practice, we use $10$-th and $90$-th percentiles as minimum and maximum values ($\text{min}\left\{\frac{1}{z_k}\right\}$  and $\text{max}\left\{\frac{1}{z_k}\right\}$) respectively, to mitigate the influence of outliers within the initialized point cloud. The $\tau$ is empirically set to $15$ for different scenes in our implementation, as the optimization process will actively update the camera parameters.

\subsection{Optimization Process} \label{sec:optimization}
We divide the entire training process into two stages: a warm-up stage and a refinement stage. In the initial $5,000$ iterations, as the Gaussian points and camera parameters undergo significant changes, we employ only $\mathcal{L}_\text{rec}$ as the training objective. This allows the Gaussian points and camera parameters to adjust to fit the training views using the DOF rendering process. After this stage, the Gaussian points and camera parameters become relatively stable, resulting in the rendered CoC map $\mathcal{M}^{(\text{coc})}$ becoming highly correlated with the pixel-wise blur extent within the training views. At this point, we begin leveraging CoC cues in conjunction with supervisions on the rendered All-in-Focus images to further refine and enhance scene details. Specifically, we introduce and use the In-Focus Localization Network (ILN) to identify in-focus regions within training views from the rendered CoC map and other information including rendered defocused image and depth map. Meanwhile, we deactivate $\mathcal{L}_\text{rec}$ and activate the remaining three terms for subsequent iterations.
 Additionally, we observe that the initial point clouds, derived from blurry images that contain multi-view inconsistent blurry regions, are sparse. The sparse initialization requires a large amount of iterations for point cloud densification to recover the fine details. To enhance the optimization efficiency and detail recovery, we add $60,000$ uniformly distributed points across the scene at the $2,000$-th iteration, a point at which the scene $S$ and camera parameters have been substantially optimized. The attributes of the newly added points are set according to its nearest neighbors. 
 We briefly summarize the optimization process in Algorithm \ref{tab:algorithm}.

 \input{tables/algorithm}
 \vspace{4mm}
\subsection{Parameter Settings and Network Structure} \label{sec:param}
\paragraph{Learning-Rate Settings}
 We set the initial learning rate for the center positions of 3D Gaussian points at $0.0005$, which linearly decays to $0.000005$ over $40,000$ iterations. The learning rate for the scales of Gaussian points is set to $0.01$. Moreover, the learning rate for focal distances is set at $0.05$, and that for aperture parameters is set to $0.01$. The In-Focus Localization Network is trained with a learning rate of $0.0005$. The remaining parameters retain the settings given in the method\cite{3dgs}.

\paragraph{Network Structure} In \Cref{tab:network}, we detail the structure of the In-Focus Localization Network (ILN). As indicated, ILN comprises four 2D convolutional layers. The first two layers are dedicated to extracting contextual information from inputs that combine the rendered CoC map $\mathcal{M}_m^{(\text{coc})}$, defocus image $\tilde{\tilde{\mathbf{I}}}_m$, and depth map $\tilde{\tilde{\mathbf{D}}}_m$. Consequently, the input to the first layer has $5$ channels, while the second layer receives $48$ channels, matching the output feature map dimension from the first layer. The third convolutional layer, which also incorporates injected positional encoding information with $48$ channels, thus receives a total of $64$ channels. The final layer receives the feature from the third layer and outputs the mask $\mathcal{M}_m^{*}$. To ensure that the output falls within the range [0,1], we apply a $\text{Sigmoid}()$ activation after the last layer.
\input{tables/table_network}

\input{figures/figure_focus_vis_2}
\section{Additional Experimental Results}
\todo{check the discussions here to see if our method sounds less attractive in the discussions.}
In this section, we provide additional experimental results. Specifically, we provide more results for focal distance analysis in \Cref{sec:ans:focus}, showcase additional qualitative results for post-capture control of focal distance and aperture parameter in \Cref{sec:ans:post_capture}, investigate the impact of training with defocused images on rendered depth-of-field effects in \Cref{sec:defocus_train}, present quantitative results and more visual results for All-in-Focus novel view synthesis in \Cref{sec:nvs}, and include visual results from the variants explored in our ablation studies in \Cref{sec:ablation}.

\subsection{Additional Results for Focal Distance Analysis} \label{sec:ans:focus}
In addition to the focal distance analysis conducted on the \emph{Cake} scene from the real defocus dataset, for which the results are provided in the main paper, we also examine the optimized focal distance parameters for training views of two additional scenes: \emph{Cupcake} and \emph{Tools}. The corresponding visualization results are presented in \Cref{fig:focus_vis2}. As shown in \Cref{fig:focus_vis2}, the focal distance parameters optimized on these two scenes closely match the manually annotated ranges of possible focal distances used during image capture. These results further demonstrate that the introduced finite-aperture camera model, combined with the proposed differentiable depth-of-field rendering process, is highly physically grounded and is able to effectively learn camera characteristics from defocused multi-view inputs.

\input{figures/figure_dof_render2}
\subsection{Additional Results for Post-Capture Control} \label{sec:ans:post_capture}
To demonstrate that our method enables depth-of-field rendering via post-capture control of aperture and focal distance parameters, we provide additional results on three scenes in \Cref{fig:dof_render2}. As shown in \Cref{fig:dof_render2}, the in-focus regions maintain sharp when the focal distance is set around their depth planes, while the out-of-focus regions demonstrate varying levels of blur with the change of aperture parameter. For instance, the fruit area in the first scene, the cookie pattern in the second scene, and the fine golden metallic structure in the third scene remain sharp at focal distances of $70$, $109$, and $48$, respectively, even as the aperture parameter $Q$ is adjusted from $101$ to values exceeding $200$ or even $300$. Meanwhile, objects at other depth planes exhibit progressively pronounced blurriness, as seen in the enlarged out-of-focus regions presented in each column. Specifically, each column highlights the effects on a single region under varying aperture parameters, effectively illustrating the depth-of-field effect achieved by our approach. It can also be observed that the positions of the in-focus and out-of-focus regions shift as the focal distance is adjusted, which allows us to achieve refocusing effects. Furthermore, simultaneously altering the focal distance and aperture parameter produces compounded effects. 

\input{figures/figure_wo_defocus_guidance}

\subsection{Influence of Training with Defocused Images} \label{sec:defocus_train}
To validate the rationale behind training our method on multi-view defocused images for achieving post-capture control of depth-of-field rendering, we examine the rendered defocused images on scenes optimized using sharp All-in-Focus images. Specifically, the synthetic scenes from the dataset \cite{ma2022deblur} provide ground-truth All-in-Focus images along with multi-view defocused images, enabling a comparative investigation. In our study, we train our approach separately on multi-view sharp images and on multi-view inconsistent defocused images. After optimization, we render defocused images from the scenes reconstructed under these two training settings. Exemplary results of the rendered defocused images from this investigation are presented in \Cref{fig:defocus_guidance}.

% As shown in \Cref{fig:defocus_guidance}, from the scene reconstructed via training on sharp images, rendering depth-of-field effects through adjusting camera parameters in our DOF rendering process results in undesired artifacts. Specifically, due to the lack of guidance from natural defocus blur in training images, the 3D Gaussian points within the scene are primarily guided for compositing sharp images for the All-in-Focus setting. Then during the depth-of-field rendering process, the Gaussian points, after convolution with separate depth-related blur kernels, fail to form natural, smooth defocus blur. Instead, the blurred Gaussian points make objects within out-of-focus regions dilated and seemingly 'enhanced'. For example, the content within the closer regions, such as the stairs, plant and 'CocaCola' text, appear increasingly dilated within the rear-focus images when the aperture parameter is increased. In the rendered near-focus images, there is no blur effects for the distant stone 柱子, which instead becomes more dilated with the aperture parameter increases and even look like a whole structure.
% The dilation effects make the objects in these regions seamingly 'enhanced', which make corresponding images fail to correctly convey the underlying focus cues.
% In contrast, the rendered rear-focus images from the scene optimized from defocused images exhibit natural, smooth defocus blur in closer regions, which effectively convey the focus information.

% Here’s a polished and refined version of your paragraph:

As shown in \Cref{fig:defocus_guidance}, depth-of-field (DOF) effects rendered from scenes reconstructed using sharp images during training exhibit undesired artifacts when camera parameters are adjusted in the DOF rendering process. Specifically, due to the absence of guidance from natural defocus blur in the training images, the 3D Gaussian points in the scene are primarily optimized to composite sharp All-in-Focus images. During the DOF rendering process, when these Gaussian points are convolved with depth-related blur kernels, they fail to generate natural and smooth defocus blur. Instead, the blurred Gaussian points cause objects in the out-of-focus regions to appear dilated and artificially "enhanced. For example, in the rear-focus rendered images, objects in closer regions, such as the stairs, the plant, and the 'Coca Cola' text, become increasingly dilated as the aperture parameter increases. Similarly, in the near-focus rendered images, the distant stone pillar does not exhibit any blur but instead becomes more dilated with increasing aperture, to the extent that it appears as a single, merged structure. These dilation effects result in a misleading "enhancement" of objects in the defocused regions, preventing the images from correctly conveying the intended depth and focus cues.

In contrast, the rear-focus and near-focus images rendered from scenes trained with defocused images exhibit natural and smooth defocus blur in closer and distant regions, respectively, effectively conveying correct focus cues. Additionally, the defocus blur adaptively changes as the aperture parameter is adjusted. This demonstrates the effectiveness of training with defocused images in achieving realistic depth-of-field rendering with our approach.

\subsection{Additional Results for All-in-Focus Novel View Synthesis} \label{sec:nvs}
\if 0
\paragraph{Results on Real dataset} As shown in \Cref{tab:real}, the performance of the state-of-the-art 3DGS-based method Mip-Splatting \cite{mip-splatting} is slightly lower than those of vanilla NeRF \cite{mildenhall2020nerf}. This phenomenon is possibly caused by the inconsistencies across views resulted from exhibited defocus blur in training views. The inconsistencies causes 3DGS-based Mip-Splatting method easier to produce more artifacts under novel views than the smooth MLP-based representations in vanilla NeRF.
The NeRF-based methods \cite{ma2022deblur, lee2023dp, peng2023pdrf} improve the performance significantly compared with vanilla NeRF, through differentiably simulating defocus blur in the rendering process. In particular, the PDRF method proposed by Peng et al. \shortcite{peng2023pdrf} achieves the highest average PSNR score (24.31 dB) and SSIM value among the methods in this line. 
However, due to the high rendering costs associated with volume rendering, these methods support rendering novel views often at speeds less than 1 fps, as reported in \cite{lee2024deblurring}.
Our method achieves PSNR and SSIM on par with PDRF, but at significantly higher framerates compared to any NeRF-based method. 
% The average SSIM performance ($0.7667$) of our method rivals that of BAGS, outperforming other methods. 
In stark contrast to concurrent 3DGS-based methods \cite{lee2024deblurring, peng2024bags}, our method simulates depth-of-field effects with the guidance of Circle-of-Confusion under learnable camera parameters including focal distance and aperture parameters, thereby also allowing for adjustable dynamic DOF rendering and refocusing of the 3D scene.
\fi 

In this section, we give comprehensive quantitative results for All-in-Focus novel view synthesis on both the real and synthetic datasets and present visual results. 

\input{figures/figure_visual_comp2}
\paragraph{Results on Real dataset}

In \Cref{tab:real}, we present the numerical results of our approach on the task of All-in-Focus novel view synthesis, comparing them against vanilla NeRF \cite{mildenhall2020nerf}, Mip-Splatting \cite{mip-splatting}, and several state-of-the-art deblur-focused methods \cite{ma2022deblur, lee2023dp, peng2023pdrf, lee2024deblurring, peng2024bags}. As shown in \Cref{tab:real}, the performance of Mip-Splatting \cite{mip-splatting} is slightly lower than that of vanilla NeRF \cite{mildenhall2020nerf}. This discrepancy arises because, although both methods produce reconstructed scenes with blurry regions caused by defocus blur, the multi-view inconsistencies introduced by defocus blur make the 3DGS-based Mip-Splatting method more prone to generating artifacts in novel views compared to the smoother MLP-based representations used in vanilla NeRF. This phenomenon is visually demonstrated in the first two rows of \Cref{fig:visual_comp2}.

NeRF-based deblur-focused methods, such as Deblur-NeRF \cite{ma2022deblur}, DP-NeRF \cite{lee2023dp}, and PDRF \cite{peng2023pdrf}, significantly improve performance compared to vanilla NeRF by differentiably simulating defocus blur during the rendering process. Among these, the PDRF method proposed by Peng et al. \shortcite{peng2023pdrf} achieves the highest average PSNR score (24.31 dB) and SSIM value. Among the 3DGS-based methods, our approach achieves comparable performance to the state-of-the-arts BAGS and Deblur-GS. Specifically, BAGS achieves highest PSNR score, our method achieves highest SSIM score. 
The visual results in \Cref{fig:visual_comp2} further demonstrate that our method is able to achieve sharp All-in-Focus renderings, suggesting that our approach effectively reconstruct the fine details from multi-view inputs with defocus blur.

\input{tables/table_real_new}
\input{figures/figure_ablation}

% The rendering speed of our method is 350 fps, which is much faster than those of NeRF-based methods and closely matches the rendering speed of Mip-Splatting. Our method achieves a lower rendering speed than BAGS, which is because the defocus blur is purely fitted by the blurred Gaussian points in our method, while it is fitted by convolvling the rendered AiF image with predicted per-pixel convolutional kernels. 
%  The rendering speed of our method, Mip-Splatting, and BAGS is generally lower than Deblur-GS due to the extra cost of anti-aliasing.
% This difference possibly makes our approach to use more points to allow for the fitting. Nevertheless, the rendering speed is much higher than $30$ fps.

% \input{figures/figure_visual_comp_syn}
% \input{tables/table_combined}
\input{tables/table_synthetic}
\todo{check the discussions here, especially on the explanations of the performance for BAGS}
\paragraph{Results on Synthetic dataset} 
In \Cref{tab:synthetic}, we present the numerical results for All-in-Focus novel view synthesis on the synthetic dataset. The performance trends are similar to those observed in the real dataset. Notably, Mip-Splatting produces a much lower average SSIM score than vanilla NeRF as it produces severe artifacts in rendered images for the \emph{Pool} scene, which is demonstrated in \Cref{fig:visual_comp2}. Regarding the BAGS method, for which the authors provide dedicated settings for each scene within the real dataset but without providing configurations for the synthetic scenes, we apply it to the synthetic dataset using a uniform configuration. Following from their configurations on  scenes from the real data, we set a relatively large number of iterations (45,000) with 9,000 dedicated to coarse-to-fine optimization. 
% but shows relatively lower performance on the \emph{Trolley} scene. 
% Attempts to adjust the iteration settings for BAGS yielded similar performance 
%
\vspace{1mm}

The PSNR and SSIM score of our method surpass those of Deblur-NeRF and DP-NeRF and are on par with the other two 3DGS-based methods, BAGS and Deblur-GS. As shown in \Cref{tab:synthetic}, the PSNR and SSIM scores for the 3DGS-based methods are slightly lower than those of the NeRF-based method PDRF \cite{peng2023pdrf}. This is likely caused by the differences in camera pose: the 3DGS-based methods, including our approach, BAGS, and Deblur-GS, rely on camera poses estimated using structure-from-motion (SfM) methods from multi-view inputs containing defocus blur. In contrast, NeRF-based methods, such as PDRF, utilize ground-truth camera poses provided by Blender. 
The visual results on synthetic scenes presented in \Cref{fig:visual_comp2} exhibit similar trends to those observed in the real dataset scenes. Our method demonstrates enhanced detail recovery compared to the NeRF-based methods and achieves comparable detail restoration to BAGS and Deblur-GS.

\subsection{Visual Results for Ablation Study} \label{sec:ablation}
In \Cref{fig:ablation},  we present the visual results from the variants examined during the ablation studies. As shown in \Cref{fig:ablation}, the absence of the detail enhancement strategy leads to results that are less sharp (e.g., the circular line and text appear blurrier compared to the outputs of our full model) or introduce artifacts, such as those visible around the ladder region. These observations highlight the effectiveness of the detail enhancement strategy in our pipeline, which is achieved by supervising rendered All-in-Focus images using Circle-of-Confusion (CoC) cues. Additionally, removing the regularization term for the predicted in-focus mask leads to reconstructed scenes with more blurry regions and artifacts. Meanwhile, it can be observed that removing the regularizer for the predicted in-focus mask,  which encourages the in-focus to be binary, makes the reconstructed scenes exhibit more blurry regions and artifacts. \Cref{fig:ablation} further demonstrates that, incorporating the loss term $\mathcal{L}_\text{mk}$ that utilizes rendered CoC maps to supervise the predicted in-focus masks, also contributes to reducing artifacts, as shown in ladder region.

% \newpage
\bibliographystyle{acmart}
{
\bibliography{reference}
}

\end{document}
